# Supplementary material for: GLAMLE: inference for multiview network data in the presence of latent variables, with application to commodities trading
Source: arXiv:2107.05915 source file (2023-01-10)
Supplement: Supplementary file 2 [file Appendix.tex]

\section{Additional Monte Carlo results for three latent variables} \label{Section: q3}
To study the impact of latent variables linear dependence,
%As was the case of one latent variable with no significant differences of results under 
we consider models with three latent variables under Assumption A2 and A2$'$. To conduct our analysis we proceed as in \S \ref{Sec: MC_gllvm} and produce similar plots, with similar interpretations. The conclusion about the bias is in line with the one of the Monte Carlo results commented in \S \ref{Sec: A2A21}. 
This is visible, for instance, 
%looking at, which displays the geometries of true and estimated response variables $\boldsymbol Y$ for A2. 
if we compare the maximum eigenvalues and three elements of the conditional means  $\hat{\boldsymbol{{\pi}}}$ and $\boldsymbol{{\pi}}_{0}$, Figure \ref{Fig: Mean_q3}-\ref{Fig: RMSE_q3} are in line with the plots in Figures \ref{Fig: Mean}-\ref{Fig: RMSE}. Also for
the three latent variable case, we notice that for A2 and A2$'$, we have similar boxplots with small bias; see e.g. Figure \ref{Fig: Mean_q3}. What's more, we obtain similar results when comparing Laplace and variational approximations shown in  Figure \ref{Fig: Mean_VA_q3}-\ref{Fig: pi_VA_q3}.

\begin{figure}[htp!]
\begin{center}
\begin{tabular}{c}  
\includegraphics[width=0.45\textwidth, height=0.27\textheight]{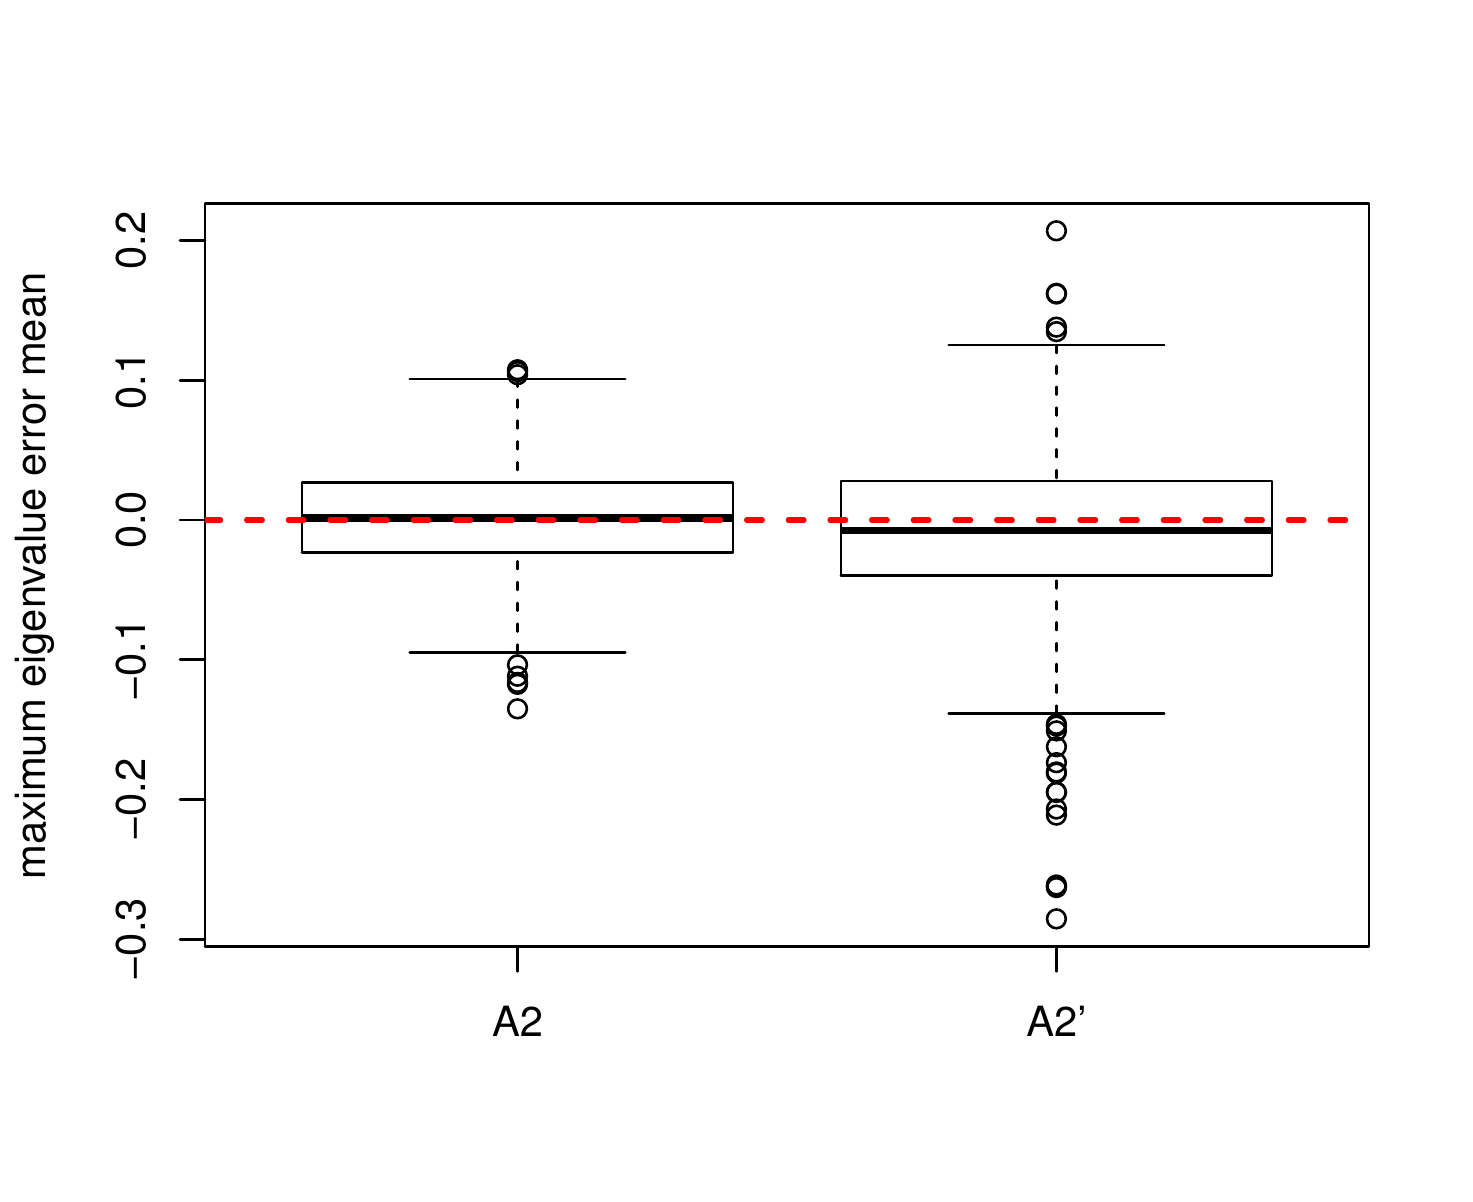}
\end{tabular}
\caption{ Bernoulli GGLLVM using Laplace approximation (LA) under Assumption A2 and A2$'$. %Left Panel: Boxplot of means of  $\hat{\boldsymbol{\pi}}-\boldsymbol{{\pi}}_{0}$. Right Panel: 
Boxplot of error means of maximum eigenvalues of  $\hat{\boldsymbol{\pi}}$ and $\boldsymbol{{\pi}}_{0}$ using three latent variable. We consider a directed graph with 18 nodes and 100 sample size. Monte Carlo size is 1000.}
    \label{Fig: Mean_q3}
\end{center}
\end{figure}

\begin{figure}[htp!]
\begin{center}
\begin{tabular}{c} 
\includegraphics[width=0.45\textwidth, height=0.3\textheight]{pi_ij_q3.eps}
\end{tabular}
\caption{Bernoulli GGLLVM using Laplace approximation (LA) under Assumption A2 and A2$'$. 
Boxplots of $\hat{\pi}^{(1)}_{ij}-\pi^{(1)}_{ij}$ for three different edges $\{ij\} \in \{11,12,13\}$ using three latent variable. We consider a directed graph with 18 nodes and 100 sample size. Monte Carlo size is 1000.}
    \label{Fig: pi_ij_q3}
\end{center}
\end{figure}

\begin{figure}[hbtp]
\begin{center}
\begin{tabular}{c} 
\includegraphics[width=0.45\textwidth, height=0.3\textheight]{RMSE_q3.eps}
\end{tabular}
\caption{Bernoulli GGLLVM using Laplace approximation (LA) under Assumption A2 and A2$'$. Boxplots of RMSEs of  $\hat{\pi}_{ij}$ for three different edges $\{ij\} \in \{11,12,13\}$ using three latent variable. We consider a directed graph with 18 nodes and 100 sample size. Monte Carlo size is 1000.}
   \label{Fig: RMSE_q3}
\end{center}
\end{figure}

\begin{figure}[hbtp]
\begin{center}
\begin{tabular}{c}  
\includegraphics[width=0.45\textwidth, height=0.27\textheight]{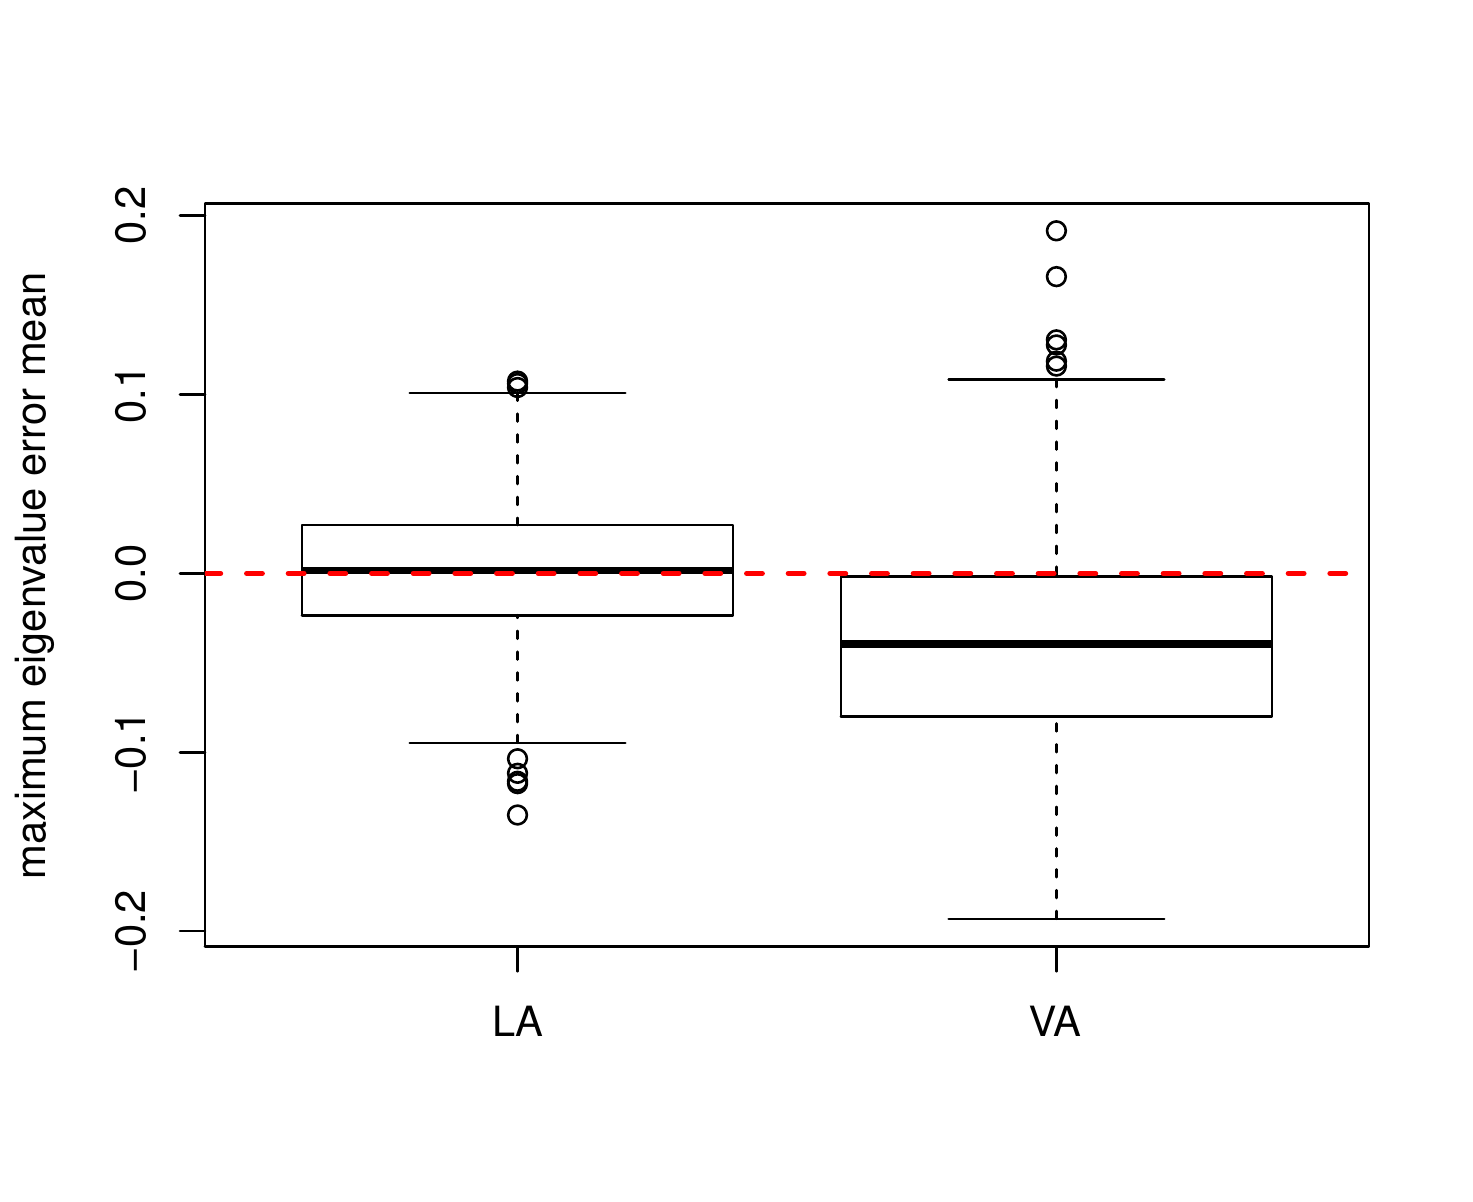}
\end{tabular}
\caption{ Comparison between Laplace approximations (LA) and variational approximations (VA) on a Bernoulli GGLLVM under Assumption A2. %Left Panel: Boxplot of means of  $\hat{\boldsymbol{\pi}}-\boldsymbol{{\pi}}_{0}$. Right Panel: 
Boxplot of error means of maximum eigenvalues of  $\hat{\boldsymbol{\pi}}$ and $\boldsymbol{{\pi}}_{0}$ using three latent variable. We consider a directed graph with 18 nodes and 100 sample size. Monte Carlo size is 1000.}
    \label{Fig: Mean_VA_q3}
\end{center}
\end{figure}

\begin{figure}[hbtp]
\begin{center}
\begin{tabular}{cc}  \hspace{0.5cm}LA & \hspace{0.5cm} VA\\
\begin{turn}
{90} \hspace{3.5cm} $q=3$
\end{turn}
\includegraphics[width=0.45\textwidth, height=0.3\textheight]{pi_LA_q3.eps}&
\includegraphics[width=0.45\textwidth, height=0.3\textheight]{pi_VA_q3.eps}\\
\end{tabular}
\caption{Bernoulli GGLLVM with one or two latent variable using Laplace approximation (LA) and variational approximation (VA), under Assumption A2. Comparison between true and estimated $\boldsymbol{\pi}^{(1)}$. We consider a directed graph with 18 nodes and 100 sample size.}
    \label{Fig: pi_VA_q3}
\end{center}
\end{figure}
